# Supplementary material for: Developing correlation-consistent numeric atom-centered orbital basis sets for Krypton: Applications in RPA-based correlated calculations
Source: arXiv:2309.06145 source file (2023-09-12)
Supplement: Supplementary file 1 [file supple_mater.pdf]

# Supporting Material for
# "Developing correlation-consistent numeric atom-centered orbital basis sets for Krypton: Applications in RPA-based correlated calculations"

Sixian Yang,[1,2] Igor Ying Zhang,[3,*] and Xinguo Ren[2,†]

[1]*Key Laboratory of Quantum Information, University of Science and Technology of China, Hefei, 230026, China*
[2]*Institute of Physics, Chinese Academy of Sciences, Beijing 100190, China*
[3]*Collaborative Innovation Center of Chemistry for Energy Materials, Shanghai, Key Laboratory of Molecular Catalysis and Innovative Materials, MOE Key Laboratory of Computational Physical Sciences, Shanghai Key Laboratory of Bioactive Small Molecules, Department of Chemistry, Fudan University, Shanghai 200433, China*

Here, the supporting materials for the main paper are presented. In Table SI, the major parameters – the effective charges $\{z_i\}$ for the NAO-VCC-$n$Z basis sets for Kr are listed. The minimal basis functions are not presented, which are the same for all NAO-VCC-$n$Z basis sets.

Figure S1 presents the frozen-core (RPA+rSE)@PBE binding energy curves of $Kr_2$ obtained using Gaussian cc-pV$X$Z basis sets with $X$ =T, Q, 5. The extrapolated CBS(Q,5) results are also included. The left and right panels show the binding energies without and with applying CP corrections. It can seen that without applying CP corrections, the binding energies of $Kr_2$ obtained with cc-pV$X$Z basis sets are one order of magnitude too big, indicating that these basis sets are contaminated with huge BSSE.

In Fig. S2, we present the binding energy curve of aug-NAO-VCC-5Z, in comparison with those obtained using NAO-VCC-5Z and Gaussian aug-cc-pV5Z basis sets. Here we use a similar strategy as aug-cc-pV5Z, adding extra diffuse basis functions of $1s1p1d1f1g1h$ as "aug" set while the original NAO-VCC-5Z basis set is kept fixed. Comparing to the cc-pV5Z results, it can be seen that adding such set of diffuse functions makes the binding strength of Kr dimer several meV stronger. In particular, the result of aug-NAO-VCC-5Z with CP correction and that of NAO-CCC-5Z without CP correction are fairly close, differing by less 2 meV at the equilibrium distance. This shows that the effects of not correcting BSSE and not including the diffuse functions for NAO-VCC-$n$Z basis sets largely cancel each other. Finally, the binding energies obtained with aug-NAO-VCC-5Z and aug-cc-pV5Z basis sets are very close, differing only by 1 meV at the equilibrium distance.

In Table. SII we present the details of the calculated RPA+rSE equilibrium volumes and cohesive energy of RPA+rSE Kr FCC bulk calculations, with NAO-VCC-4Z and 5Z basis sets, as well as the CBS(4,5) results. The purpose here is to check the effect of counterpoise corrections for the periodic bulk. For a FCC primitive cell that contains only one atom, there are totally 12 first nearest neighbors of a given atom, and 6 second-nearest neighbors. Tests show that it is sufficient to consider only the 12 nearest neighbors of the central atom, and the change in CP correction energy is smaller than 1 meV if one further takes the 6 second-nearest neighbors into account. Hence, the CP correction energy is given by evaluating the energy difference between the isolated atom and the atom surrounded by its 12 nearest-neighbor ghost atoms with bond lengths corresponding to a specific atomic volume. We confirm that the BSSE error amounts to about 9 meV at the CBS(4,5) level in the RPA calculations. However, it is also shown that there is sizable BSSE error in the rSE part, giving rise to a total 24 meV CP correction energy. The Birch–Murnaghan fit of the CP corrected curve gives equilibrium volume and cohesive energy of RPA+rSE Kr FCC bulk 47.55 $\AA^3$(5.750$\AA$) and -112.1 meV, respectively, slightly overestimating the lattice constant by 0.08 $\AA$ and underestimating the cohesive energy by 9.7 meV.

---

* igor_zhangying@fudan.edu.cn

† renxg@iphy.ac.cn

TABLE SI. The major parameters – the effective nuclear charge $z_i$ of hydrogen-like orbitals for the $(sp)$correlation subset and polarization subset in the NAO-VCC-$n$Z$(n = 2, 3, 4, 5)$ basis sets for Kr. The minimal basis is not presented here.

| NAO-VCC-2Z | | NAO-VCC-3Z | |
|---|---|---|---|
| $(sp)$correlation | $\{z_i\}$ | $(sp)$correlation | $\{z_i\}$ |
| $(1s)$ | 1.892 | $(2s)$ | 1.446, 1.536 |
| $(1p)$ | 3.777 | $(2p)$ | 5.071, 5.325 |
| Polarization | | Polarization | |
| $(1d)$ | 5.709 | $(2d)$ | 5.901, 5.952 |
| | | $(1f)$ | 9.701 |

| NAO-VCC-4Z | | NAO-VCC-5Z | |
|---|---|---|---|
| $(sp)$correlation | $\{z_i\}$ | (sp)correlation | $\{z_i\}$ |
| $(3s)$ | 1.379, 2.180, 3.447 | $(4s)$ | 1.623, 1.943, 2.326, 2.784 |
| $(3p)$ | 3.989, 4.588, 5.278 | $(4p)$ | 5.065, 5.872, 6.809, 7.895 |
| Polarization | | Polarization | |
| $(3d)$ | 6.183, 7.810, 9.865 | $(4d)$ | 6.462, 7.399, 8.471, 9.698 |
| $(2f)$ | 9.251, 9.313 | $(3f)$ | 11.992, 12.667, 13.380 |
| $(1g)$ | 14.105 | $(2g)$ | 14.326, 14.567 |
| | | $(1h)$ | 20.347 |

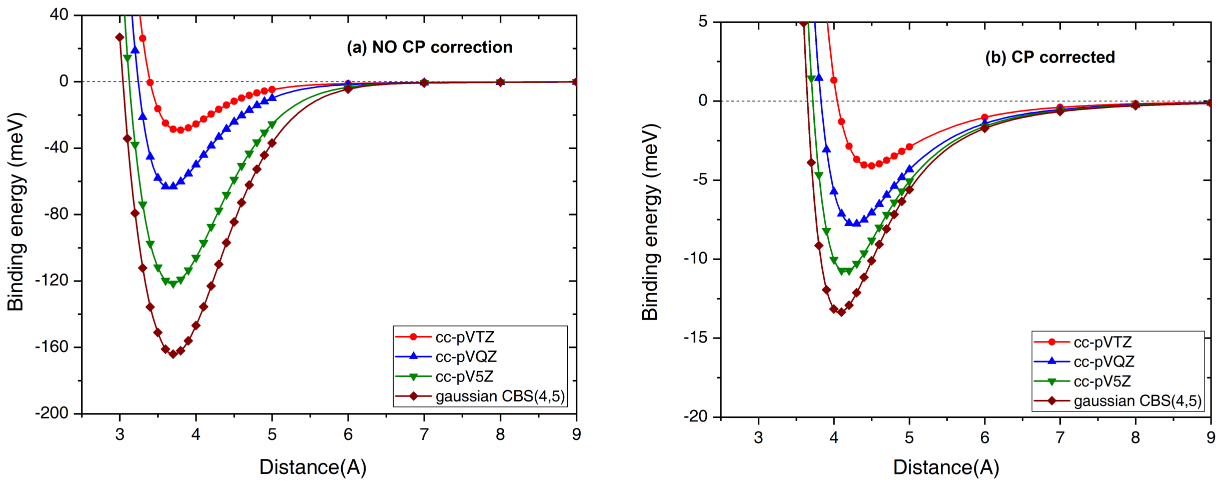


FIG. S1. (RPA+rSE)@PBE binding energy curves of the Kr dimer obtained using Gaussian cc-pV$XZ$ basis sets ($X$=T, Q, 5), as well as the extrapolated CBS(4,5) results. The left and right panels show the results without and with CP corrections, respectively.

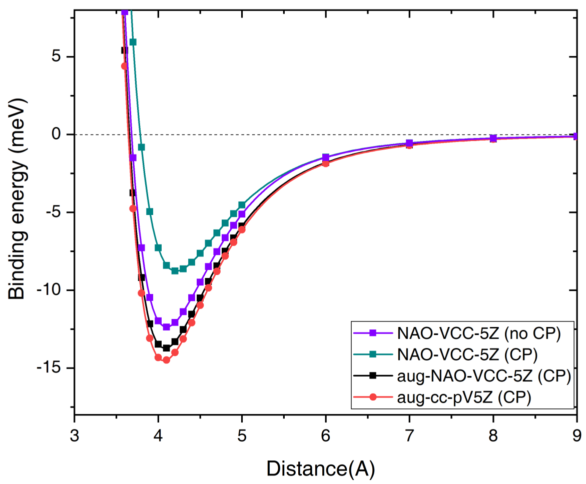


FIG. S2. Binding energy curve of $Kr_2$ via aug-NAO-VCC-5Z basis set and aug-cc-pV5Z gaussian basis set with CP corrections. The aug-NAO-VCC-5Z basis set consists of one extra diffuse basis function per each angular momentum channel, compared to NAO-VCC-5Z. The results of NAO-VCC-5Z with or without CP correction are also shown for comparison.

TABLE SII. RPA and RPA+rSE equilibrium volumes and cohesive energies given by second-order Birch–Murnaghan fit for Kr FCC bulk, with or without CP corrections. Results obtained using NAO-VCC-4Z and 5Z basis sets, as well as the CBS(4,5) results, are shown. The unit of volume and cohesive energy is Å$^3$ and meV, respectively.

| Basis set | no CP correction | | CP corrected | |
|---|---|---|---|---|
| | $V_{eq}$ | $E_{eq}$ | $V_{eq}$ | $E_{eq}$ |
| RPA | | | | |
| NAO-VCC-4Z | 49.39 | -59.35 | 52.63 | -46.81 |
| NAO-VCC-5Z | 48.79 | -79.97 | 51.62 | -69.07 |
| NAO-VCC CBS(4,5) | 48.18 | -101.73 | 50.54 | -92.63 |
| RPA+rSE | | | | |
| NAO-VCC-4Z | 45.71 | -85.29 | 49.23 | -61.79 |
| NAO-VCC-5Z | 45.15 | -110.13 | 48.39 | -86.25 |
| NAO-VCC CBS(4,5) | 44.67 | -136.31 | 47.55 | -112.11 |
